# Supplementary material for: What Challenges Do Developers Face About Checked-in Secrets in Software Artifacts?
Source: arXiv:2301.12377 source file (2023-01-29)
Supplement: Supplementary file 1 [file Appendix.tex]

\input{Tables/QuestionCountPerYear}
\input{Tables/tagskeywords}
\newcolumntype{s}{>{\hsize=0.03\hsize}X}
\newcolumntype{b}{>{\hsize=0.75\hsize} X}
\newcolumntype{m}{>{\hsize=0.15\hsize}X}
\begin{table*}
\centering
\caption{Answer to RQ2. The mapping of answers to each question category}
\label{question-answer-mapping}
\footnotesize
%\tiny
\begin{tabularx}{\textwidth} {|s|m|b|}
\hline
\multicolumn{1}{|c|}{\textbf{Domain}} & \multicolumn{1}{l|}{\textbf{Question Category}} & \multicolumn{1}{c|}{\textbf{Answer Category}} \\ \hline \hline
\multirow{5}{*}{Secrets}
 & Q1: Store/Version & Revokation and Rotation, Move Secrets out of Source Code/Version Control and Use Template Config File, Secret Management in Deployment (Deployment Variables, Config Transformations), Use of External Secret Management Service (HashiCorp Vault and Azure key Vault), Use Local Environment Variables, Restrict API Access and Permissions, Load Externally and Use Secondary Private Repository, Server-Side Implementation \\ \cline{2-3}
 
 & Q2: Ignore/Hide & Revokation and Rotation, Rewrite VCS History (Use git-filter-branch, git-filter-repo and BFG repo cleaner), Move Secrets out of Source Code/Version Control and Use Template Config File, VCS Feature (Git Hooks: Git attribute custom driver, pre-commit and post-commit hooks), Store Encrypted/Obfuscated Secrets, Secret Management in Deployment (Deployment Variables, Config Transformations, Shared Directory), Use of External Secret Management Service (HashiCorp Vault and Azure key Vault), Use Local Environment Variables, Load Externally and Use Secondary Private Repository, Server-Side Implementation\\ \cline{2-3}
 
  & Q3: Exploitability & Revokation and Rotation, Rewrite VCS History (Use of git-filter-branch), Move Secrets out of Source Code/Version Control and Use Template Config File \\ \cline{2-3}
 
 & Q4: Distribute & Move Secrets out of Source Code/Version Control and Use Template Config File, Secret Management in Deployment, Load Externally and Use Secondary Private Repository \\ \cline{2-3}

 & Q5: Restriction & Restrict API Access and Permissions \\ \hline
 
   \multirow{4}{*}{\begin{tabular}[l]{@{}l@{}}Deploy-\\ment\end{tabular}} 
 & Q6: Store/Version & Move Secrets out of Source Code/Version Control and Use Template Config File, VCS Feature (Git attribute custom driver), Store Encrypted/Obfuscated Secrets, Secret Management in Deployment (Config Transformation, Deployment Variables, Configuration Management Systems (Puppet, Ansible-Vault)), Use of External Secret Management Service (HashiCorp Vault, Azure Key Vault), Use Local Environment Variables, Restrict API Access and Permissions, Load Externally (S3) and Use Secondary Private Repository, Server-Side Implementation \\ \cline{2-3} 
 
  & Q7: Improper Configuration & Move Secrets out of Source Code/Version Control and Use Template Config File, Secret Management in Deployment (Deployment Tools: GitHub Actions, Deployment Variables), External Secret Management Service (AWS Secret Manager), Use Local Environment Variables
\\ \cline{2-3}
 
 & Q8: Ignore/Hide & Move Secrets out of Source Code/Version Control and Use Template Config File, Store Encrypted/Obfuscated Secrets (Mask Passwords Plugin), Secret Management in Deployment (Deployment Variables, Keep dot file out of root directory), Use of External Secret Management Service (Azure key Vault), Use Local Environment Variables
\\ \cline{2-3}

 & Q9: Dot File  & Secret Management in Deployment (Keep dot file out of root directory) \\ \hline
 
 \multirow{4}{*} {\begin{tabular}[l]{@{}l@{}}VCS \\Feature\end{tabular}} 
  & Q10: History Sanitize & Revokation and Rotation, Rewrite VCS History (Use git-filter-branch, git-filter-repo, BFG repo cleaner, git reset --hard, git rebase), Move Secrets out of Source Code/Version Control and Use Template Config File, VCS Scan Tools (Truffle Hog, Gitrob), Load Externally and Use Secondary Private Repository
 \\ \cline{2-3} 
 
  & Q11: Ignore Already Committed  & Rewrite VCS History, Move Secrets out of Source Code/Version Control and Use Template Config File, VCS Feature (Git Flags: git --skip-worktree, git update-index --assume-unchanged), Use Local Environment Variable \\ \cline{2-3}
  
  & Q12: Line Level Security & Move Secrets out of Source Code/Version Control and Use Template Config File, VCS Feature (Git Hooks: Git attribute custom driver, pre-commit and post-update hook), Add Files to the Staging Area Explicitly, Store Encrypted/Obfuscated Secrets (Rails Secrets), Use Local Environment Variables, Load Externally and Use Secondary Private Repository
 \\ \cline{2-3}
  
   & Q13: Encrypt File & VCS Feature (Git Hooks: pre-commit and post-commit) \\ \hline
 
 \multirow{5}{*} {\begin{tabular}[l]{@{}l@{}}Configur-\\ ation File\end{tabular}}   
 & Q14: Store/Version & Move Secrets out of Source Code/Version Control and Use Template Config File, Store Encrypted/Obfuscated Secrets, Secret Management in Deployment (Deployment Variables, Config Transformations, Shared Directory), Use of External Secret Management Service, Use Local Environment Variables, Load Externally and Use Secondary Private Repository \\ \cline{2-3}  
 
  & Q15: Ignore/Hide & Move Secrets out of Source Code/Version Control and Use Template Config File, Add Files to the Staging Area Explicitly, Store Encrypted/Obfuscated Secrets, Secret Management in Deployment, Use Local Environment Variables, Load Externally and Use Secondary Private Repository\\ \cline{2-3}
  
 & Q16: Distribute &  Move Secrets out of Source Code/Version Control and Use Template Config File \\ \cline{2-3}
    
    & Q17: Exploitability & Use Local Environment Variables, Use of External Secret Management Service, Move Secrets out of Source Code/Version Control and Use Template Config File \\ \cline{2-3}
    
     & Q18: Accessibility & Secret Management in Deployment (Config Transformation) \\ \hline
     
      \multirow{1}{*}{\begin{tabular}[l]{@{}l@{}}Pre-open\\ Source\end{tabular}} 
 & Q19: Cross-check & Rewrite VCS History (Use of git-filter-branch, git-filter-repo, BFG repo cleaner), Move Secrets out of Source Code/Version Control and Use Template Config File, Store Encrypted/Obfuscated Secrets, Secret Management in Deployment (Deployment Variables, Mask Secrets in log), Use of External Secret Management Service (Cloud KMS), Use Local Environment Variables, Load Externally and Use Secondary Private Repository, Server-Side Implementation \\ \hline
     
  \multirow{3}{*} {\begin{tabular}[l]{@{}l@{}}Client- \\Side\\Applicat-\\ion\end{tabular}} 
  & Q20: Store & Revokation and Rotation, Store Encrypted/Obfuscated Secrets, Use Local Environment Variables, Move Secrets out of Source Code/Version Control and Use Template Config File, Server-Side Implementation
\\ \cline{2-3} 
  
  & Q21: Hide & Revokation and Rotation, Use Local Environment Variables, Move Secrets out of Source Code/Version Control and Use Template Config File, Server-Side Implementation \\ \cline{2-3}
  
  & Q22: Exploitability  & Move Secrets out of Source Code/Version Control and Use Template Config File \\ \hline
  
    \multirow{2}{*}{\begin{tabular}[l]{@{}l@{}}Secure-\\ness\end{tabular}} 
 & Q23: Private Repository & Use of External Secret Management Service, Move Secrets out of Source Code/Version Control and Use Template Config File, Load Externally and Use Secondary Private Repository
\\ \cline{2-3}
 
  & Q24: Unpushed Branch & Move Secrets out of Source Code/Version Control and Use Template Config File \\ \hline
 
  \multirow{2}{*}{\begin{tabular}[l]{@{}l@{}}Ext. Sec. \\ Mng.. \end{tabular}} 
 & Q25: Setup  & Load Externally and Use Secondary Private Repository \\
 &   & \\\hline
  
  \multirow{2}{*}{Others} 
 & Q26: Importance & No Accepted Answer \\ \cline{2-3}
 
  & Q27: Decision  & Revokation and Rotation\\ 
  \hline
     
\end{tabularx}
\end{table*}
